# Supplementary material for: Topology-aware Serverless Function-Execution Scheduling
Source: arXiv:2205.10176 source file (2023-07-06)
Supplement: Supplementary file 1 [file appendix.tex]

\section{Testing details}
\label{sec:appendix}
In this section, we report the details on the testing cluster from
\cref{sec:testing} and the numeric data of the tests presented in \cref{fig:overhead_tests,fig:datalocality_tests} in \cref{sec:results}.

\cref{tab:t2,tab:t3} shows the specifications of the nodes of the testing
cluster (AWS and Azure) and \cref{tab:t1} contains the latency between the Azure
and AWS instances described in \cref{sec:test_environment} (calculated sending a
\textit{ping} command with 100 requests), and their respective specifications.

In \crefrange{tab:t4}{tab:t12} the columns correspond to, from left to right,
vanilla OpenWhisk, and the \textit{default}, \textit{isolated},
\textit{min\_memory}, and \textit{shared} distribution policies. All cells,
besides the last one report, separated by a semicolon, 1) the aggregate, average
latency of a single run of the related test (run following the configuration
from \cref{sec:test_environment}) and 2) the standard deviation of the average.
The cells in the last row contain the average of the averages of the other cells
in the same column and, separated by a semicolon, the standard deviation of such
average.

% \cref{fig:tapp_tests} reports the \tapp script used in the tests: the tag \texttt{locality} in the script was used by all data-locality tests: \textbf{mongoDB}, \textbf{terrain}, and \textbf{data-locality}.

% \vfill\eject

\begin{table*}[t]
	\centering
	% \resizebox{\columnwidth}{!}{
		\pgfplotstabletypeset[NormalStyle]{csv/cluster.csv}
		% }
	\caption{\label{tab:t2}CPU and memory specifications for Azure instances.}
\end{table*}

\begin{table*}[h]
	\centering
	% \resizebox{\columnwidth}{!}{
		\pgfplotstabletypeset[NormalStyle]{csv/services.csv}
		% }
	\caption{\label{tab:t3}CPU and memory specifications for AWS instances.}
\end{table*}

\begin{table*}[t]
	\centering
	\resizebox{\columnwidth}{!}{\pgfplotstabletypeset[NormalStyle]{csv/ping.csv}}
	\caption{\label{tab:t1}Latency statistics between Azure and AWS instances.}
	\end{table*}

\begin{table*}[h]
	\centering
	\pgfplotstabletypeset[NormalStyle,ResultsStyle]{csv/results/single_runs/hellojs.csv}
	\caption{\label{tab:t4}Results for the runs of the \textbf{hellojs} test case.}
\end{table*}

\begin{table*}[h]
	\centering
	\pgfplotstabletypeset[NormalStyle,ResultsStyle]{csv/results/single_runs/matrixMult.csv}
	\caption{\label{tab:t5}Results for the runs of the \textbf{matrixMult} test case.}
\end{table*}

\begin{table*}[h]
	\centering
	\pgfplotstabletypeset[NormalStyle,ResultsStyle]{csv/results/single_runs/sleep.csv}
	\caption{\label{tab:t6}Results for the runs of the \textbf{sleep} test case.}
\end{table*}

\begin{table*}[h]
	\centering
	
	\pgfplotstabletypeset[NormalStyle,ResultsStyle]{csv/results/single_runs/cold-start.csv}
	\caption{\label{tab:t7}Results for the runs of the \textbf{cold-start} test case.}
\end{table*}

\begin{table*}[h]
	\centering
	\pgfplotstabletypeset[NormalStyle,ResultsStyle]{csv/results/single_runs/slackpost.csv}
	\caption{\label{tab:t8}Results for the runs of the \textbf{slackpost} test case.}
\end{table*}

\begin{table*}[h]
	\centering
	\pgfplotstabletypeset[NormalStyle,ResultsStyle]{csv/results/single_runs/pycatj.csv}
	\caption{\label{tab:t9}Results for the runs of the \textbf{pycatj} test case.}
\end{table*}

\begin{table*}[h]
	\centering
	\pgfplotstabletypeset[NormalStyle,ResultsStyle]{csv/results/single_runs/terrain.csv}
	\caption{\label{tab:t10}Results for the runs of the \textbf{terrain} test case.}
\end{table*} 

\begin{table*}[h]
	\centering
	\pgfplotstabletypeset[NormalStyle,ResultsStyleData]{csv/results/single_runs/mongoDB.csv}
	\caption{\label{tab:t11}Results for the runs of the \textbf{mongoDB} test case.}
\end{table*} 

\begin{table*}[h]
	\centering
	\pgfplotstabletypeset[NormalStyle,ResultsStyleData]{csv/results/single_runs/data-locality.csv}
	\caption{\label{tab:t12}Results for the runs of the \textbf{data-locality} test case.}
\end{table*}

% \begin{figure*}[t]
% 	\begin{lstlisting}[language=yaml,numbers=left,showlines,backgroundcolor=\color{Gold1!20},mathescape=true]
% default:
%  - workers: ~*~
%    strategy: ~platform~
%    invalidate: ~max_concurrent_invocations~: ~100~
% locality:
%  - controller: ~US_Controller~
%    topology_tolerance: ~all~
%  		workers: ~*~
%    strategy: ~random~
%    invalidate: ~max_concurrent_invocations~: ~100~
% 	\end{lstlisting}
% 	\caption{\label{fig:tapp_tests}\tapp script used in the experiments.}
% \end{figure*}

% \begin{figure*}[h]
% 	\begin{lstlisting}[language=yaml,numbers=left,showlines,backgroundcolor=\color{Gold1!20},mathescape=true]
% default:
%  - workers: ~*~
%    strategy: ~platform~
%    invalidate:
%     - ~max_concurrent_invocations~: ~100~
%     - ~capacity_used~: ~50~
% locality:
%  - controller: ~US_Controller~
%    topology_tolerance: ~all~
%  		workers: ~*~
%    strategy: ~random~
%    invalidate:
%     - ~max_concurrent_invocations~: ~100~
%     - ~capacity_used~: ~50~
% 	\end{lstlisting}
% 	\caption{\tapp script used in the experiments.}
% \end{figure*}
